# Supplementary material for: Non-Primary Channel Access in IEEE 802.11 UHR: Comprehensive Analysis and Evaluation
Source: arXiv:2403.11300 source file (2024-05-12)
Supplement: Supplementary file 1 [file appendix.tex]

\subsection{Appendix 1}\label{app:1}
